# Supplementary material for: Numerical-experimental observation of shape bistability of red blood cells flowing in a microchannel
Source: arXiv:1711.06986 source file (2017-11-19)
Supplement: Supplementary file 1 [file SI.pdf]

# Supplementary information for “Numerical-experimental observation of shape bistability of red blood cells flowing in a microchannel”

Achim Guckenberger[a] Alexander Kihm[b] Thomas John,[b] Christian Wagner,[b c] Stephan Gekle[a]

Dated: November 19, 2017

## Contents

S1 Croissant and slipper initial shapes 1

S2 Time evolution details 2

S3 About the error bars in the prediction 3

S4 Additional experimental data 5

S5 References 5

S6 Raw experimental images at $x = 10\,\text{mm}$ 7

S7 Raw experimental images at $x = 0\,\text{mm}$ 12

## S1 Croissant and slipper initial shapes

Figure S1 shows the employed red blood cell (RBC) shapes when the initial shape is taken to be a croissant or slipper. These shapes were obtained from a previous simulation where we started with the typical discocyte shape. Figure S2 depicts the corresponding simulation setups, which are identical to the one from the main text except for the different RBC shape. Especially note that the initial radial offset $r_{\text{init}}$ of the centroid is along the same line. We always use the same croissant or slipper shape, regardless of the value of $r_{\text{init}}$.

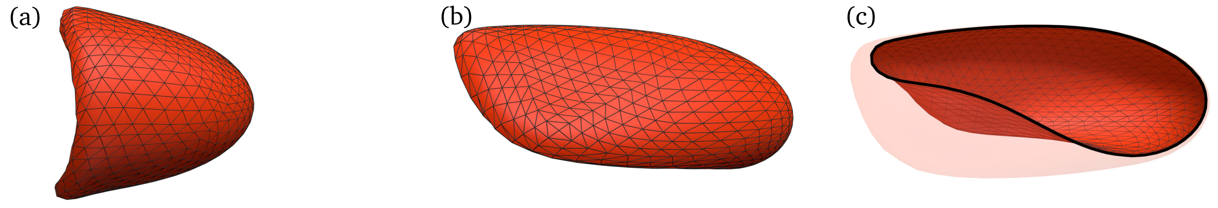


Figure S1: Employed initial shapes in the simulations when starting as a (a) croissant or (b) slipper. Figure (c) shows the cross-section of the slipper from (b). The black lines on the surfaces represent the used mesh.

[a]Biofluid Simulation and Modeling, Fachbereich Physik, Universität Bayreuth, Bayreuth
[b]Experimental Physics, Saarland University, 66123, Saarbrücken, Germany
[c]Physics and Materials Science Research Unit, University of Luxembourg, Luxembourg, Luxembourg

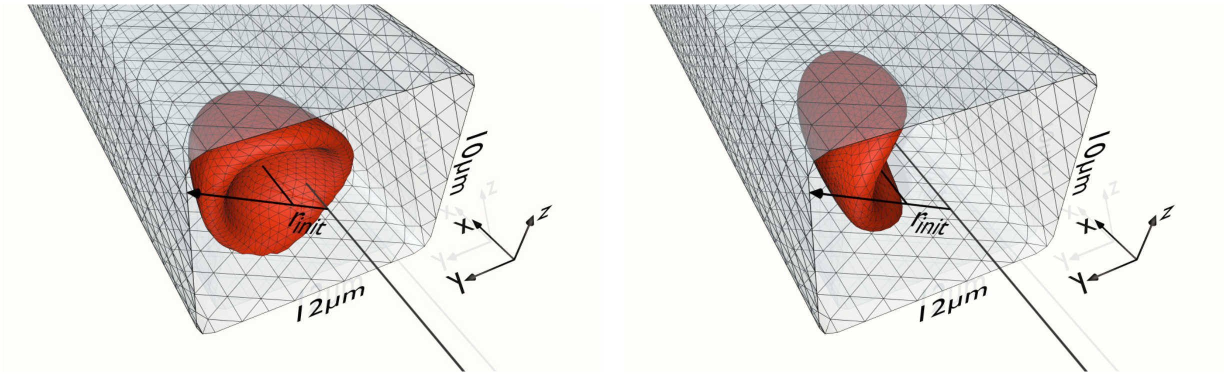


Figure S2: The simulation setups when starting with a croissant (left) or a slipper shape (right), similar to figure 2 from the main text. The cell shapes are the ones from figure S1.

## S2 Time evolution details

As noted in the main text and shown in the `TTSlipper` supplementary video, the tank-treading (TT) slipper exhibits oscillatory contractions. These result in periodic variations of the radial position and the cell velocity, as exemplified in figure S3. This figure also illustrates how we extract the average, minimal and maximal values after reaching the steady state. The simulation results from the main text depict the average values as the main data points and the minimal and maximal values via error bars. Note that we do the same for the other shapes, although the resulting error bars are too small to be seen in the figures.

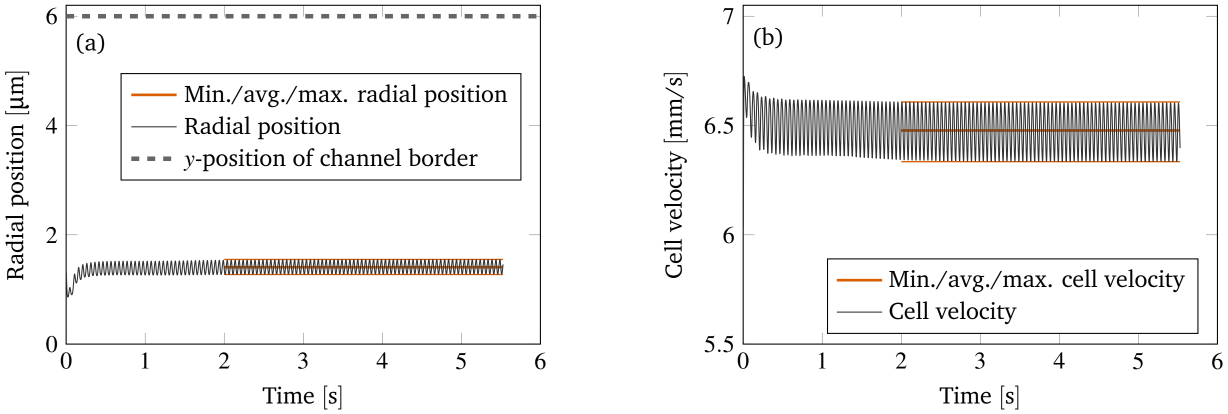


Figure S3: Time evolution of (a) the radial position and (b) the cell velocity for a slipper shape. The data is for the numerical simulation with $r_{\text{init}} = 1.2\,\mu\text{m}$ from figure 5 in the main text. The orange lines show from bottom to top the minimum, average and maximum values that are extracted in the steady state, which is taken to begin at 2 s in this particular example.

Furthermore, reaching the steady state often takes a few seconds. Convergence into the croissant shape usually takes longer than reaching a steady slipper state. This is illustrated in figure S4(a) where we show for each simulation from figure 6 in the main text the approximated time until the steady state is reached. This time is the duration measured from the start of the simulations until the position, shape, velocity and deformation of the cells no longer change or become periodic. The longest times are observed when the velocity lies in the croissant-only range. An example for such a case is displayed in figure S4(b): For around eight seconds, the cell is in an almost periodic slipper state before moving to the center and becoming a croissant. However, after another four seconds some membrane rotation occurs, i.e. the RBC dimples (which are special points due to the discocyte reference state) move to a slightly different location. This results in a short lived and slightly off-centered position. After a total time of around 14 s the cell is in the final croissant state, with no movement occurring anymore. See the video `LongCroissant` for an illustration.

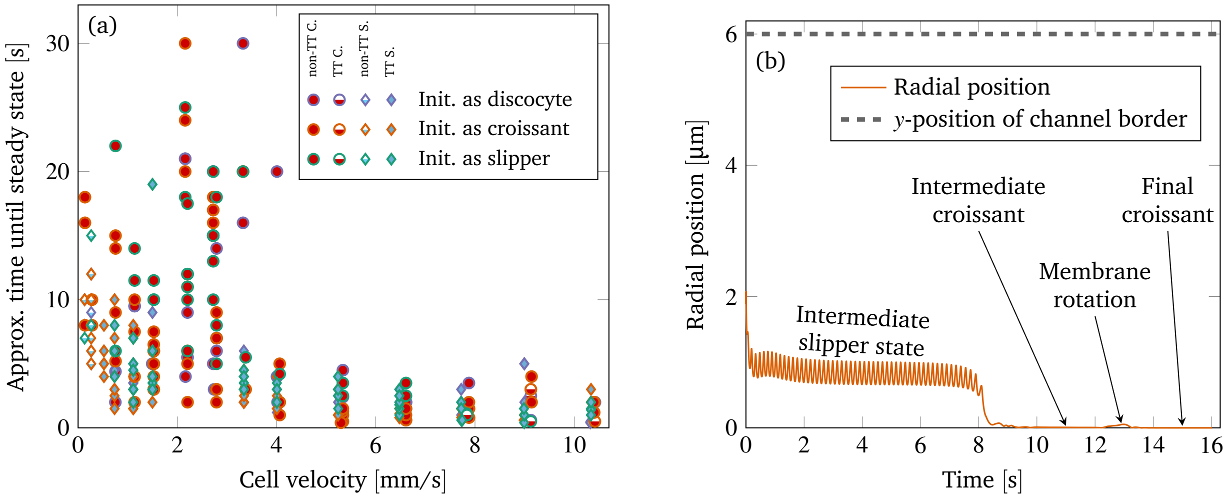


Figure S4: (a) Estimates of the time it takes for the cells to reach the steady state. The figure shows this time for all simulations from the three diagrams from figure 6 in the main text, where the cell was initialized as discocyte, croissant and slipper, respectively. These three initial shapes are indicated by the purple, orange and green borders around the symbols (see the three rows in the legend). The final steady state shapes (non-tank-treading croissant, tank-treading croissant, non-tank-treading slipper and tank-treading slipper) are represented by the same symbols as in the main text (compare the four columns in the legend). (b) Time evolution of the radial position of a cell which is initially in the discocyte state with $r_{\text{init}} \approx 1.89\,\mu\text{m}$ and has an average velocity of $\approx 2.79\,\text{mm/s}$ in the steady state (i.e. it lies in the croissant-only region). The steady state begins at around 14 s. See the movie `LongCroissant` for a 3D visualization.

# S3 About the error bars in the prediction

The determination of the vertical error bars in the comparison between experiments and simulations (figure 8 in the main text) consists of several steps that will be described in the following. To this end, consider figure S5. This figure shows exemplarily the numerical phase diagram when the starting shape is the discocyte, i.e. the symbols that indicate the steady states are identical to figure 6(a) from the main text. The middle gray line represents the position of the approximated transition threshold $r_{\text{trans}}$ between croissants and slippers, which was obtained by averaging the values from the adjacent simulation symbols.

The first step in the determination of the vertical error bars is to compute a lower and upper bound for the transition threshold. We do this by drawing a line through the highest croissant and lowest slipper symbols. This leads to the lower violet and upper green lines in figure S5. Thus, these two lines represent the uncertainty of the transition, which is a result of the finite distance between the simulations.

An exception in the construction of the three lines occurs in the region where the simulations predict only croissants. Due to the particular starting shape, there is a maximal initial offset. Experimentally, however, it is of course possible that the cells at the channel entrance have a larger offset (i.e. one that lies above the black dashed line in figure S5). Since the results from the simulations indicate that only croissants really exist in this region (regardless of the initial shape and offset), we take $r_{\text{trans}} \to \infty$. That way we predict a value of 1 for the fraction of croissants.

Second, we need to evaluate the transition lines at the experimental velocities. However, the measured velocities have not only an average $u$ but also a certain standard deviation $\sigma_u$. $\sigma_u$ is taken as the uncertainty in the velocity here. Evaluating the middle gray line at the average velocity $u$ results in the "best guess for $r_{\text{trans}}$" (the circular symbols in figure S5). This value is then directly converted into the predicted fraction of croissants $\phi$ as described in the main text (via conversion to $y_{\text{trans}}$ and the measured offset distribution at the channel entrance). For the vertical error bars, we evaluate the three numerical transition lines (lower, middle and upper, i.e. violet, gray and green) at the three velocities $u$, $u - \sigma_u$ and $u + \sigma_u$, leading to nine values for $r_{\text{trans}}$. The ones that will yield the lowest and largest fraction of croissants are shown as triangular symbols in figure S5 (the "lowest guess for $r_{\text{trans}}$" and the "largest guess for $r_{\text{trans}}$").

Third, the predicted fractions of croissants are computed from the offset distribution at the channel entrance for each of these nine $r_{\text{trans}}$ values (as described in the main text), and additionally for $r_{\text{trans}} \pm s_{\text{P}}$. This takes into account the uncertainty in the offset distribution due to the uncertainty $s_{\text{P}}$ in the position measurement. As a result, we now have 27 predictions.

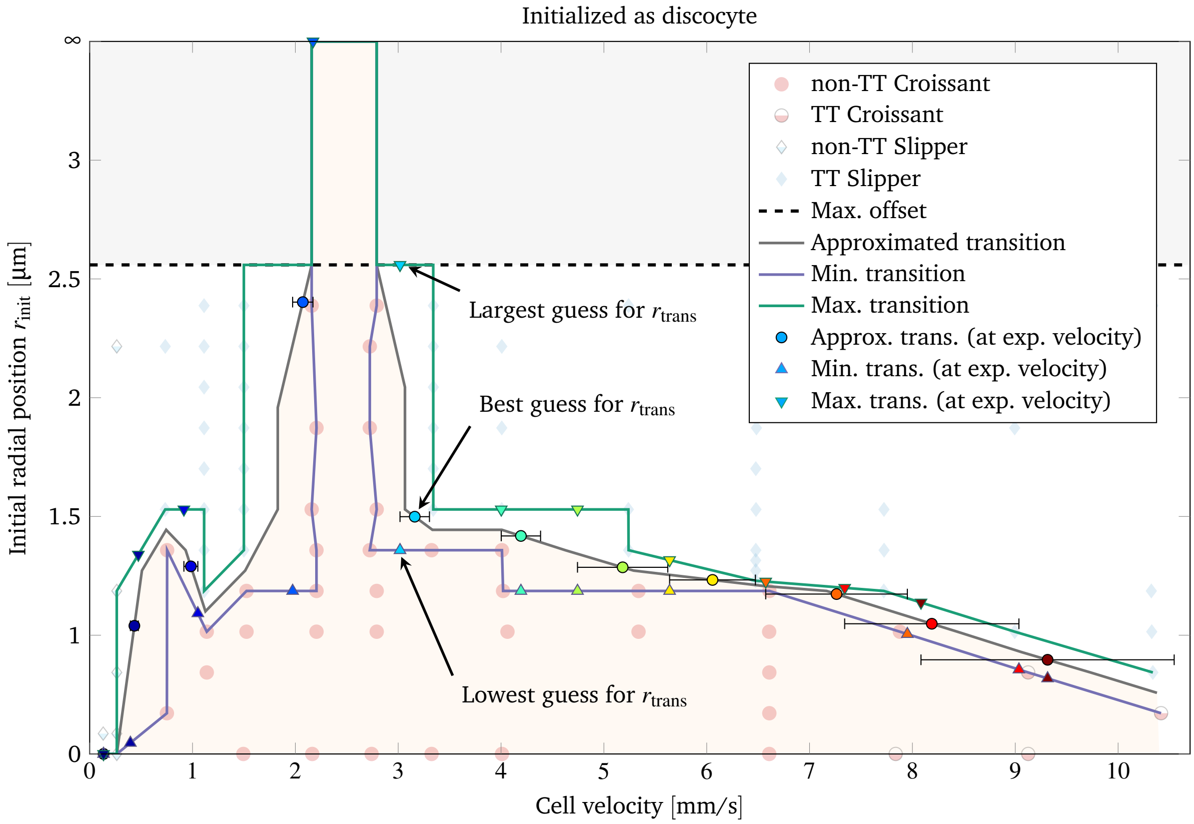


Figure S5: Numerical phase diagram from figure 6(a) from the main text for the discocyte starting shape. The nearly transparent shape symbols and the maximal offset are identical to figure 6(a). The violet, gray and green lines depict the minimal, average and maximal position, respectively, of the transition threshold $r_{trans}$ between croissants and slippers. These lines are evaluated at the experimental velocities $u$ and $u \pm \sigma_u$, giving the circular and triangular symbols. Each triple of these symbols that shares the same color corresponds to one particular experimental velocity and shows the lowest, best and largest guess for $r_{trans}$. This is exemplified via the three labels and arrows for $u \pm \sigma_u = (3.16 \pm 0.14)$ mm/s which corresponds to a pressure drop of $\Delta P = 300$ mbar. The horizontal error bars depict $\sigma_u$. Also note that in the croissant-only region we take $r_{trans} \to \infty$, as indicated by the $\infty$ symbol on the top left.

Fourth, we search for the minimum ($\phi_{\text{min}}$) and maximum ($\phi_{\text{max}}$) of these 27 values. $\phi_{\text{min}}$ and $\phi_{\text{max}}$ are then interpreted as the uncertainty in the prediction. The vertical error bars in figure 8 from the main text therefore depict $\phi_{\text{min}}$ and $\phi_{\text{max}}$.

All of this is performed not only for the phase diagram with the discocyte, but also for the ones with the croissant and slipper starting shapes. In case of the croissant starting shape, $r_{\text{trans}}$ is not a proper function due to the protrusions, i.e. we find several transition offsets for certain velocities (compare figure 6 in the main text). Hence, the simple "counting of cells that enter with an offset below $r_{\text{trans}}$" to form the prediction becomes a "counting of cells that enter with offsets in the intervals formed by the numerical transition offsets". As an example, if a certain velocity leads to transitions at $r_1$, $r_2$ and $r_3$ (such that the simulations yield croissants in the two intervals $[0, r_1]$ and $[r_2, r_3]$), then we count how many cells enter the channel with an offset that lies in these two intervals (after their projection on the $y$-axis). The computation of the uncertainty is adapted accordingly.

# S4 Additional experimental data

We depict in figure S6 the measured cell velocities for each applied pressure drop $\Delta P$. The data shows the result when the averaging goes over all cells regardless of their shape ("All"), and also for the three shape classes separately. Obviously, the cell velocities are roughly proportional to $\Delta P$. However, croissants tend to be a bit faster than slippers because croissants are located in the high-velocity center of the channel while slippers are off-centered (see the main text). This is in agreement with previous publications [1, 2].

Table S1 lists the corresponding raw data, as well as the number of cells that were taken into account. It additionally shows the number of cells at the channel entrance. The raw images from the experiments are included in sections S6 and S7 below.

Furthermore, we list in an extra Excel sheet (`SI_rawYPos_pos0.xls`) the raw $y$-positions of the cells at the channel entrance. This data makes it possible to compare one's own simulation results with our experiments (as we did in figure 8 in the main text).

Moreover, figure S7 depicts the experimental $y$-offset distributions separated into the contributions from the three different shapes (croissants, slippers and "others") at position $x = 10$ mm in the channel. This figure complements figure 3(b) from the main text where all three shapes have been considered together.

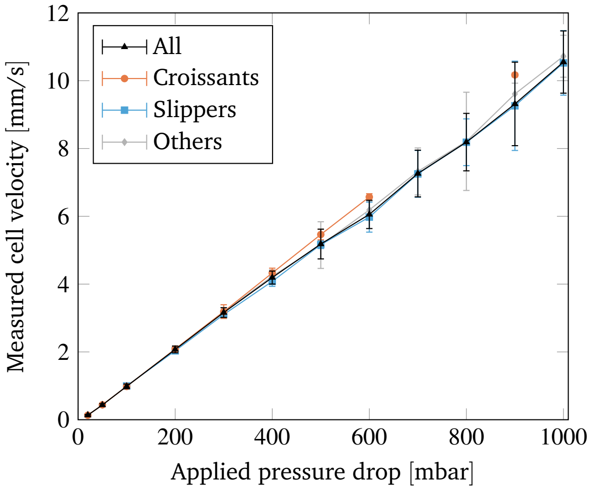


Figure S6: Measured average cell velocities for each applied pressure drop for the three different shape classes and once for all shapes together ("All"). The vertical error bars depict the standard deviation $\sigma_u$. Measurements performed at position $x = 10$ mm in the channel. The corresponding raw data is listed in table S1. The lines are guides for the eyes.

# S5 References


[1] S. Quint, A. F. Christ, A. Guckenberger, S. Himbert, L. Kaestner, S. Gekle, and C. Wagner, *"3D tomography of cells in micro-channels,"* Appl. Phys. Lett. **111**, 103701 (2017).

[2] G. Tomaiuolo, M. Simeone, V. Martinelli, B. Rotoli, and S. Guido, *"Red blood cell deformation in microconfined flow,"* Soft Matter **5**, 3736 (2009).

| $\Delta P$ [mbar] | $N_0^{\text{all}}$ | $N_{10}^{\text{all}}$ | $N_{10}^{\text{Crois}}$ | $N_{10}^{\text{Slipper}}$ | $N_{10}^{\text{Other}}$ | $u_{10}^{\text{all}}$ [mm/s] | $u_{10}^{\text{Crois}}$ [mm/s] | $u_{10}^{\text{Slipper}}$ [mm/s] | $u_{10}^{\text{Other}}$ [mm/s] |
|---|---|---|---|---|---|---|---|---|---|
| 20 | 35 | 107 | 9 | 0 | 98 | $0.135 \pm 0.021$ | $0.132 \pm 0.020$ | | $0.135 \pm 0.021$ |
| 50 | 10 | 52 | 9 | 0 | 43 | $0.43 \pm 0.04$ | $0.440 \pm 0.005$ | | $0.43 \pm 0.04$ |
| 100 | 29 | 205 | 165 | 2 | 38 | $0.98 \pm 0.07$ | $0.98 \pm 0.07$ | $0.996 \pm 0.002$ | $0.99 \pm 0.04$ |
| 200 | 71 | 484 | 252 | 22 | 210 | $2.07 \pm 0.10$ | $2.09 \pm 0.08$ | $2.03 \pm 0.06$ | $2.06 \pm 0.12$ |
| 300 | 95 | 475 | 102 | 120 | 253 | $3.16 \pm 0.14$ | $3.19 \pm 0.20$ | $3.10 \pm 0.09$ | $3.18 \pm 0.13$ |
| 400 | 90 | 463 | 80 | 167 | 216 | $4.19 \pm 0.19$ | $4.33 \pm 0.14$ | $4.08 \pm 0.15$ | $4.23 \pm 0.19$ |
| 500 | 179 | 215 | 17 | 117 | 81 | $5.2 \pm 0.4$ | $5.46 \pm 0.16$ | $5.16 \pm 0.11$ | $5.2 \pm 0.7$ |
| 600 | 151 | 176 | 8 | 124 | 44 | $6.1 \pm 0.4$ | $6.57 \pm 0.10$ | $6.0 \pm 0.4$ | $6.19 \pm 0.25$ |
| 700 | 159 | 123 | 0 | 105 | 18 | $7.3 \pm 0.7$ | | $7.3 \pm 0.7$ | $7.3 \pm 0.7$ |
| 800 | 75 | 200 | 0 | 169 | 31 | $8.2 \pm 0.8$ | | $8.2 \pm 0.7$ | $8.21 \pm 1.40$ |
| 900 | 187 | 282 | 2 | 241 | 39 | $9.3 \pm 1.2$ | $10.17 \pm 0.06$ | $9.3 \pm 1.3$ | $9.6 \pm 0.3$ |
| 1000 | 141 | 305 | 0 | 266 | 39 | $10.6 \pm 0.9$ | | $10.5 \pm 1.0$ | $10.7 \pm 0.6$ |

Table S1: Experimental data: The table lists for each applied pressure drop $\Delta P$ the total number of analyzed cells $N_0^{\text{all}}$ at position $x = 0$ mm in the channel and the total number of analyzed cells $N_{10}^{\text{all}}$ at position $x = 10$ mm. For the latter we also show the number of croissants, slippers and "others", together with the measured velocities $u_{10}$. The uncertainties are the standard deviation. The subscripts "0" and "10" in the heading specify the $x$-position in the channel (0 mm or 10 mm).

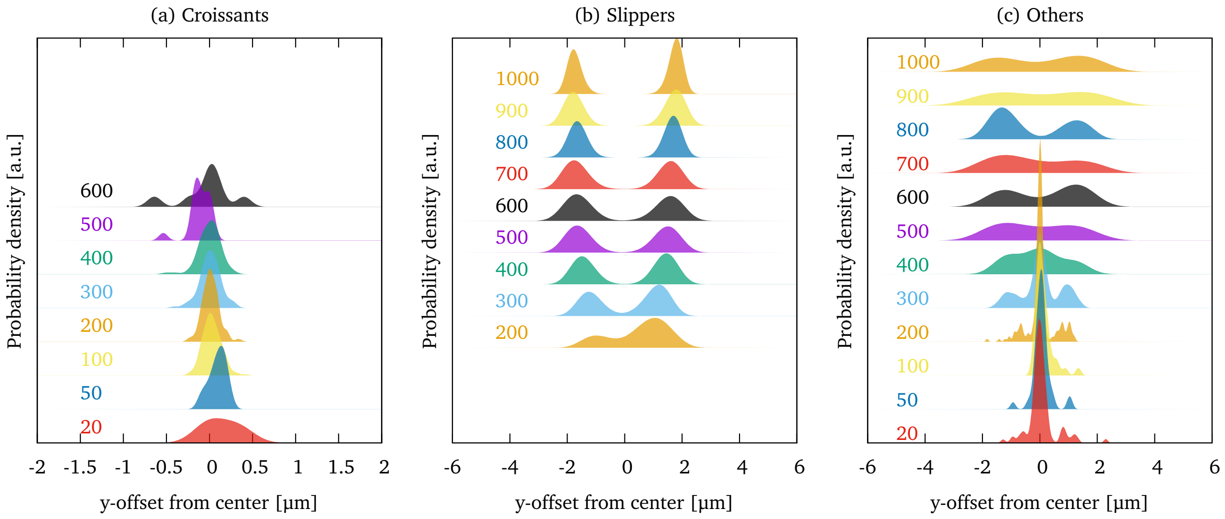


Figure S7: Estimated probability density functions for the experimental $y$-offset distributions at position $x = 10$ mm in the channel for (a) the croissant, (b) the slipper and (c) the "other" shapes. The result for all three shapes combined was shown in figure 3(b) in the main text. The area below each curve is normalized to 1, and they are offset in the vertical direction for illustration purposes. Also note the different scale of the horizontal axis in the first figure.

## S6 Raw experimental images at $x = 10\,\mathrm{mm}$

Note: The images in the individual collections are ordered from centered to off-centered.
Note: Many of the “others” (e.g. for $\Delta P = 200\,\mathrm{mbar}$) might be croissants, but they can also be slippers that are viewed from the “top” (i.e. when camera would point along the $z$-direction, one might see slippers). Since we cannot decide this from these images, we classify them as “others”.

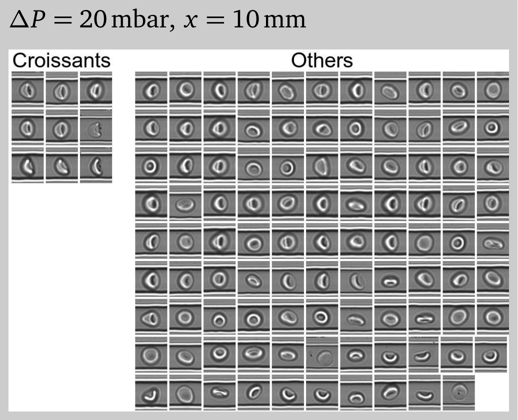


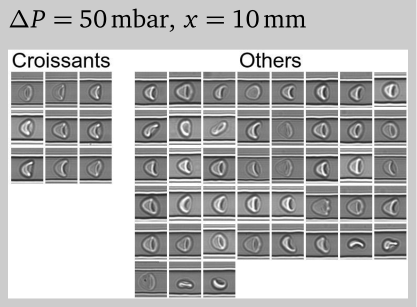


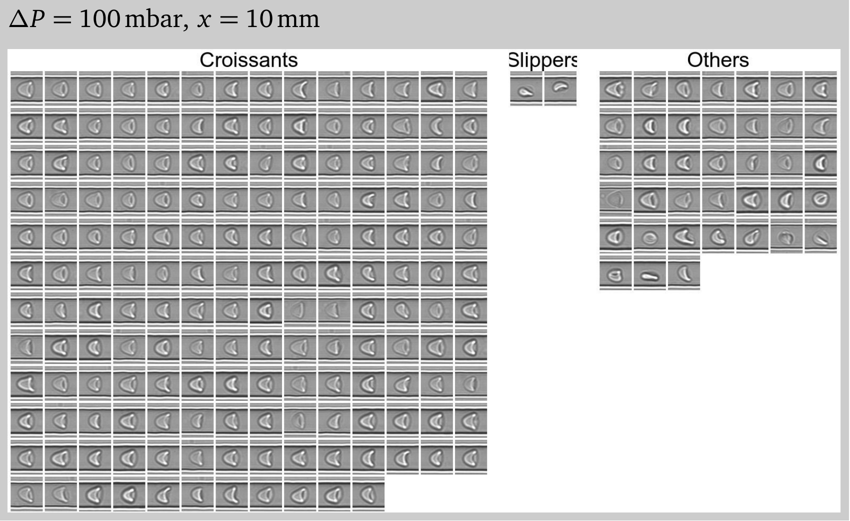

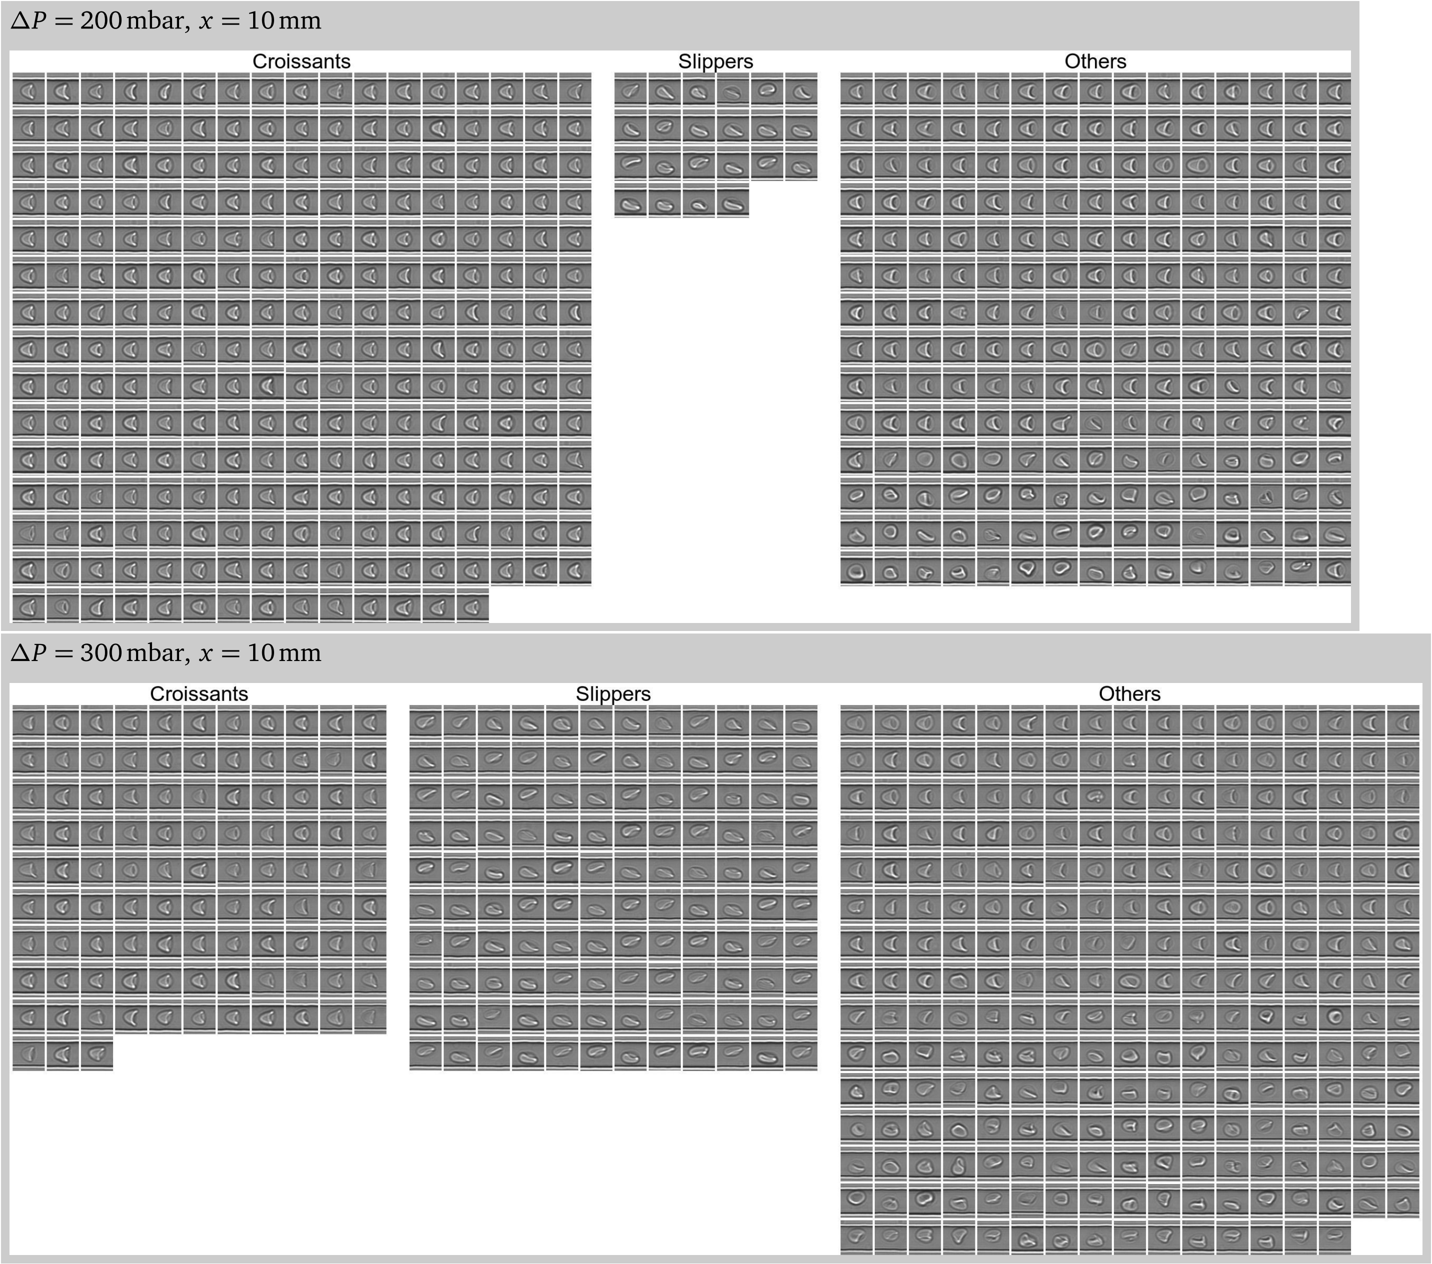

ΔP = 200 mbar, x = 10 mm
Croissants
Slippers
Others
ΔP = 300 mbar, x = 10 mm
Croissants
Slippers
Others

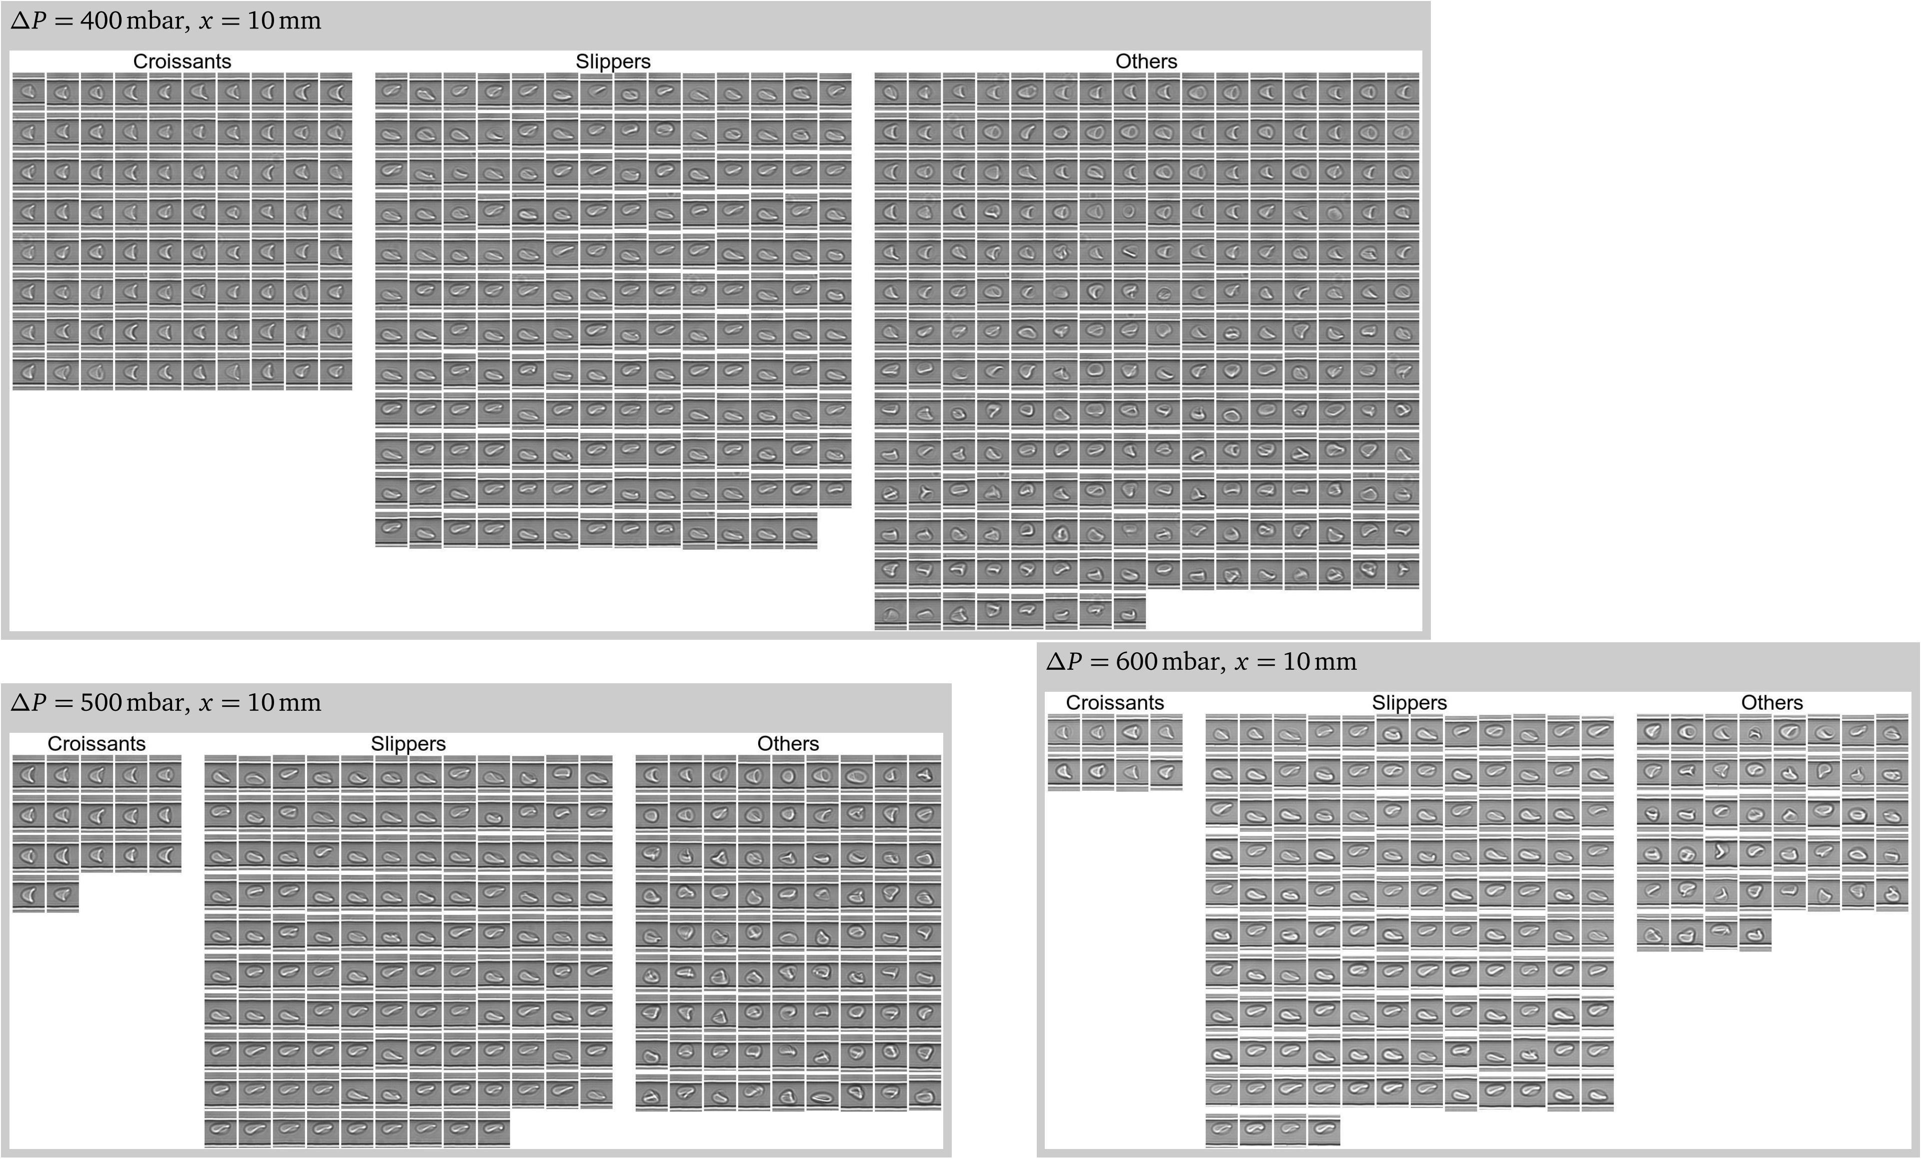

$\Delta P = 400\,\mathrm{mbar}$, $x = 10\,\mathrm{mm}$
Croissants
Slippers
Others
$\Delta P = 500\,\mathrm{mbar}$, $x = 10\,\mathrm{mm}$
Croissants
Slippers
Others
$\Delta P = 600\,\mathrm{mbar}$, $x = 10\,\mathrm{mm}$
Croissants
Slippers
Others

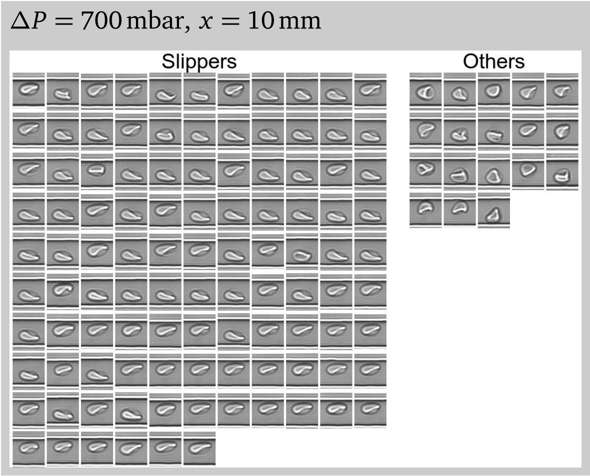
$\Delta P = 700\,\mathrm{mbar},\ x = 10\,\mathrm{mm}$
Slippers
Others

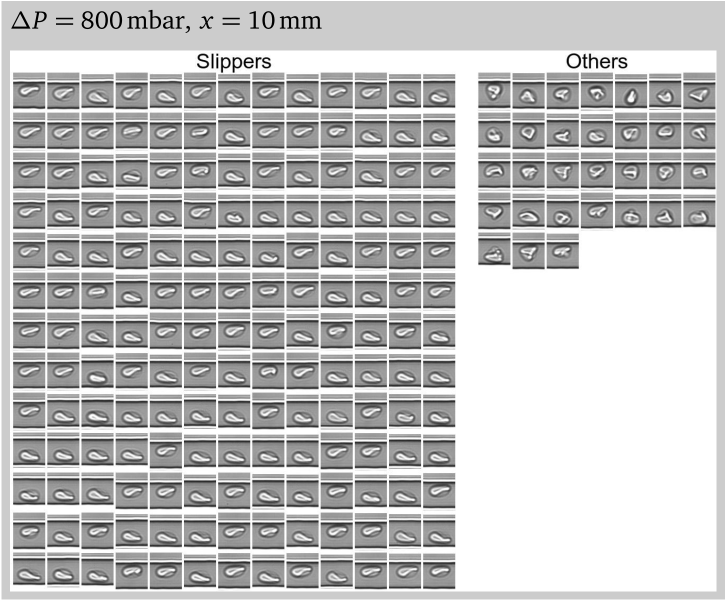
$\Delta P = 800\,\mathrm{mbar},\ x = 10\,\mathrm{mm}$
Slippers
Others

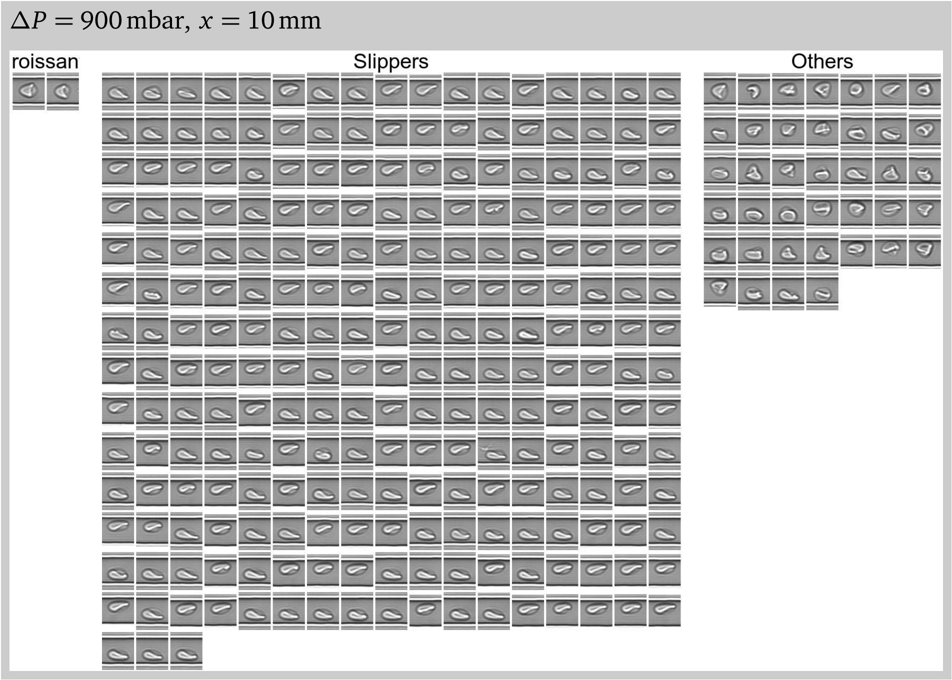
$\Delta P = 900\,\mathrm{mbar},\ x = 10\,\mathrm{mm}$
roissan
Slippers
Others

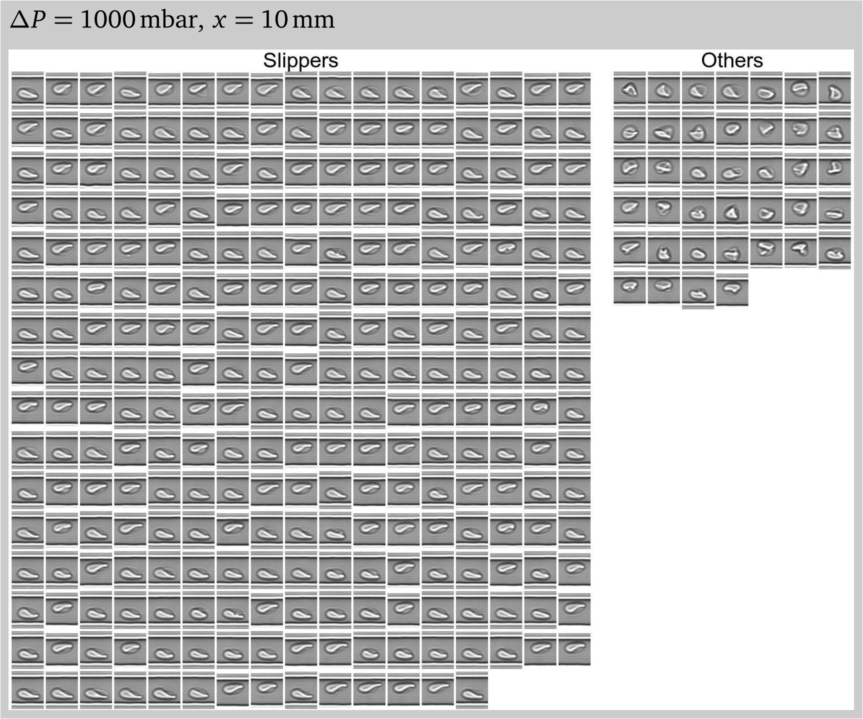
$\Delta P = 1000\,\mathrm{mbar},\ x = 10\,\mathrm{mm}$
Slippers
Others

## S7 Raw experimental images at $x = 0\,\mathrm{mm}$

Note: The images in the individual collections are ordered from centered to off-centered.

$\Delta P = 20\,\mathrm{mbar}$, $x = 0\,\mathrm{mm}$

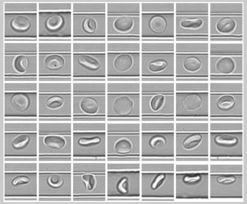

$\Delta P = 50\,\mathrm{mbar}$, $x = 0\,\mathrm{mm}$

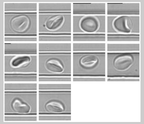

$\Delta P = 100\,\mathrm{mbar}$, $x = 0\,\mathrm{mm}$

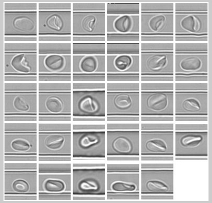

$\Delta P = 200\,\mathrm{mbar}$, $x = 0\,\mathrm{mm}$

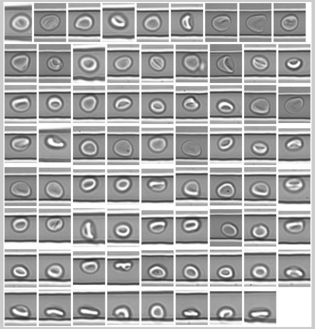

$\Delta P = 300\,\mathrm{mbar}$, $x = 0\,\mathrm{mm}$

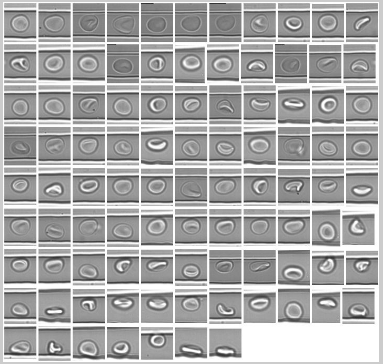

$\Delta P = 400\,\mathrm{mbar}$, $x = 0\,\mathrm{mm}$

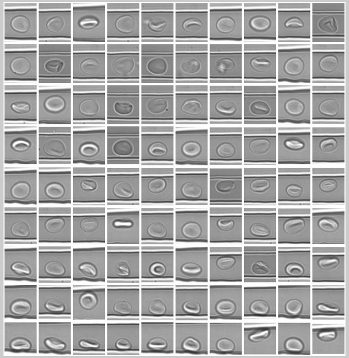

$\Delta P = 500\,\mathrm{mbar}$, $x = 0\,\mathrm{mm}$

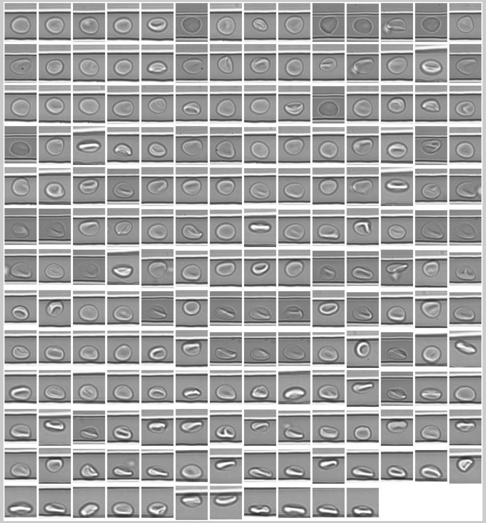

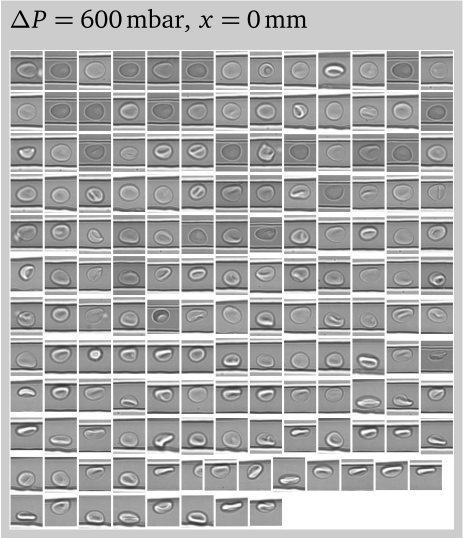
$\Delta P = 600\,\mathrm{mbar},\ x = 0\,\mathrm{mm}$

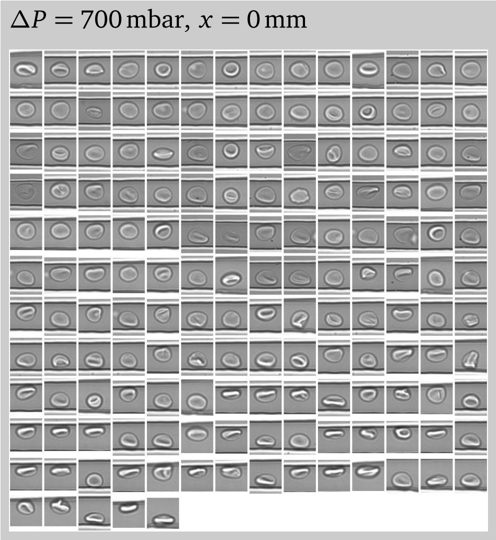
$\Delta P = 700\,\mathrm{mbar},\ x = 0\,\mathrm{mm}$

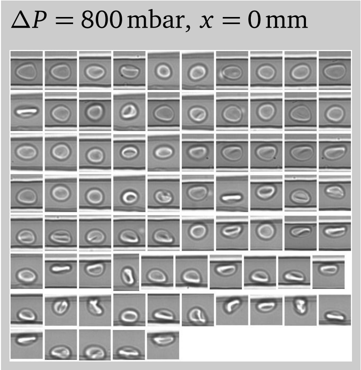
$\Delta P = 800\,\mathrm{mbar},\ x = 0\,\mathrm{mm}$

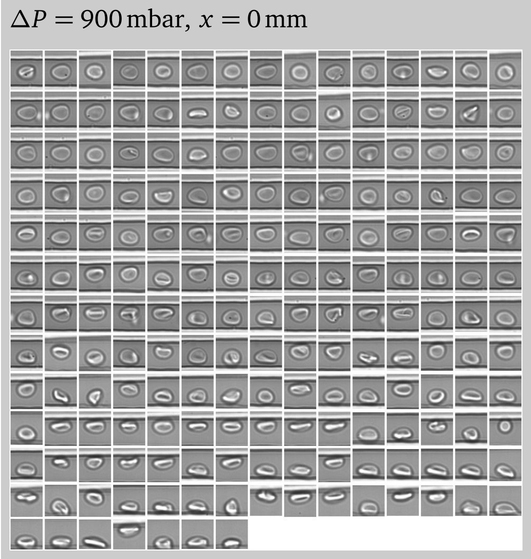
$\Delta P = 900\,\mathrm{mbar},\ x = 0\,\mathrm{mm}$

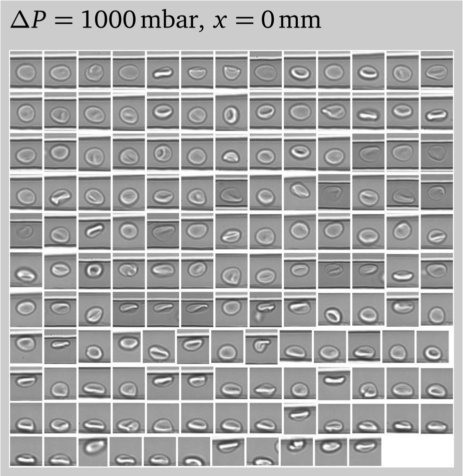
$\Delta P = 1000\,\mathrm{mbar},\ x = 0\,\mathrm{mm}$
